# Supplementary material for: VecFlow: A High-Performance Vector Data Management System for Filtered-Search on GPUs
Source: arXiv:2506.00812 source file (2025-06-01)
Supplement: Supplementary file 1 [file _s7_appendix.tex]

% Analysis
%   - The effectiveness of our optimizations
  
%     -- Zero redundant clustering
    
%         -- Naive clustering based CAGRA (memory bloat issue)
        
%         -- Zero redundancy (much more memory efficient)
        
%         -- Similar speed (?) (higher speed than unfiltered search)
        
%     -- BFS
    
%         -- Naive BFS
        
%         -- Refinement-based BFS
        
%    -- (P1) Effectiveness over different data scale
%       -- 1M vs. 10M, 100M
%    -- (P1) batch size analysis, 1 (persistent kernel), 1K, massive. 
%    -- (P2) Dimensionality, 128, 960
   
%    -- (P3) Sequential search (Big + Small) vs. Parallel search (Big + Small)
   
%    -- (p1/p2) Distribution of labels (50 labels vs. 200k labels)

% abstract: 0.25 pages

% Intro: 1-1.5 pages

% background: 0.5 page

% Motivation:

% - Application/Scenarios: ads, multimodal

% - Filtered search leads to low recall (inlined filter, 0.8 recall)

% - Naive GPU-based filtered search (post-processing) leads prolonged latency 

% Design: 3-4 pages

% - Big + small: specificity

%     - Big: zero-redundancy clustering index + CAGRA search(Jingyi)
    
%       -- Index construction
      
%          -- Data layout and design of zero-redundancy clustering-based CAGRA (Jingyi)
         
%          -- (P1): Adaptive outdegree R (Jingyi)
         
%       -- Search
      
%         -- Large-batch 
        
%         -- Small-batch: persistent kernel (Ben will check with the PK author about their plan)
        
%         -- Single CTA vs. multiple CTA
        
%     - Small: Refinement-based BFS search (Chenghao)
    
%       -- Index construction
      
%       -- Search
      
% - (P1) Single label vs. multi label

% - Put it together (Chenghao, Jingyi)

%   -- Parameter selection: specificity threshold
  
%   -- How much should go with the big index, and how much goes to the BFS.
  
%   -- (P3): Parallel search using CUDA core + TensorCore
  
%   -- Performance analytic model: memory bandwidth and compute analysis
  
% Evaluation: 3-4 pages
  
% Related work: 0.25-0.5 pages

% Conclusion: 0.25
